# Supplementary material for: Near-field plasmonics for generation of phonon lasing in a thermal nanomachine
Source: arXiv:2112.15170 source file (2022-06-14)
Supplement: Supplementary file 1 [file SM.pdf]

**Supplementary Information**

## Table 1: Photonic and plasmonic waveguide

| **Waveguide Dimensions** | |
|---|---|
| *Si waveguide length (z), width (x)* | 0.5 µm, 450 nm |
| *Si waveguide thickness (y)* | 250 nm |
| *Au film thickness* | 60 nm |
| *Taper /Au/$SiO_2$/Si length* | 330 nm |
| *Au, $SiO_2$, Si tip width* | 20 nm |
| *$SiO_2$ thickness* | 10 nm |
| *HeatSink (Au) length, width* | 222 nm, 450 nm |
| *HeatSink thickness* | 250 nm |
| *Metal cladding length, width* | 50 nm, 450 nm |
| *Metal cladding thickness* | 100 nm |

## Table 2: Film thicknesses and parameters used in Optical/Thermal Simulations

| **Film (thickness)** | **Refractive Index (830 nm)** | **Heat Capacity ($J\cdot m^{-3}K^{-1}$)** | **Thermal Conductivity ($W\cdot m^{-1}K^{-1}$)** |
|---|---|---|---|
| *Heated Air/Lubricant (10 nm)* | 1.4+0.01i | $1.0\times10^{6}$ | 3.0 |
| *InGaAs QD Layers (30 nm)* | 3.57+0.24i | $5.94\times10^{3}$ | 0.14 |
| *Heat Sink (66 nm)* | 3.72+3.99i | $3.06\times10^{6}$ | 10.5 |
| **Materials (NFT, waveguide)[29]** | | | |
| *Gold* | 0.06+5.17i | $2.49\times10^{6}$ | 317 |
| *$SiO_2$* | 1.45 | $1.6\times10^{6}$ | 1.4 |
| *Si* | 3.67 | $1.63\times10^{6}$ | 131 |
| *Metal cladding* | 2.14+4.24i | $3.73\times10^{6}$ | 3.0 |

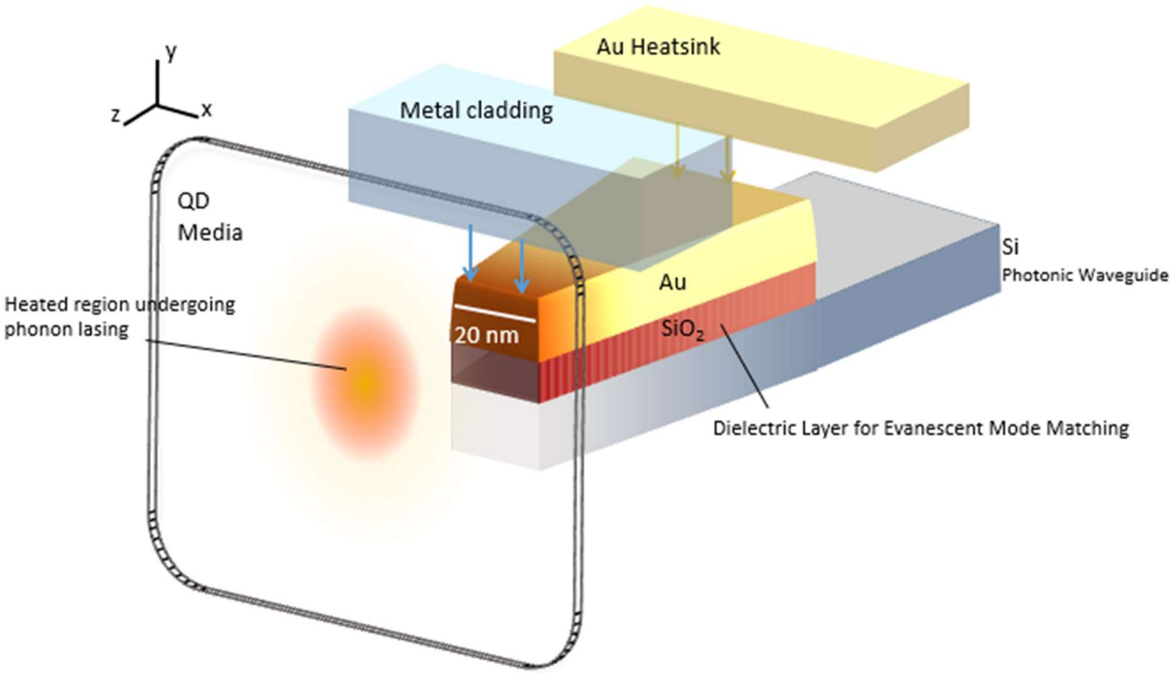


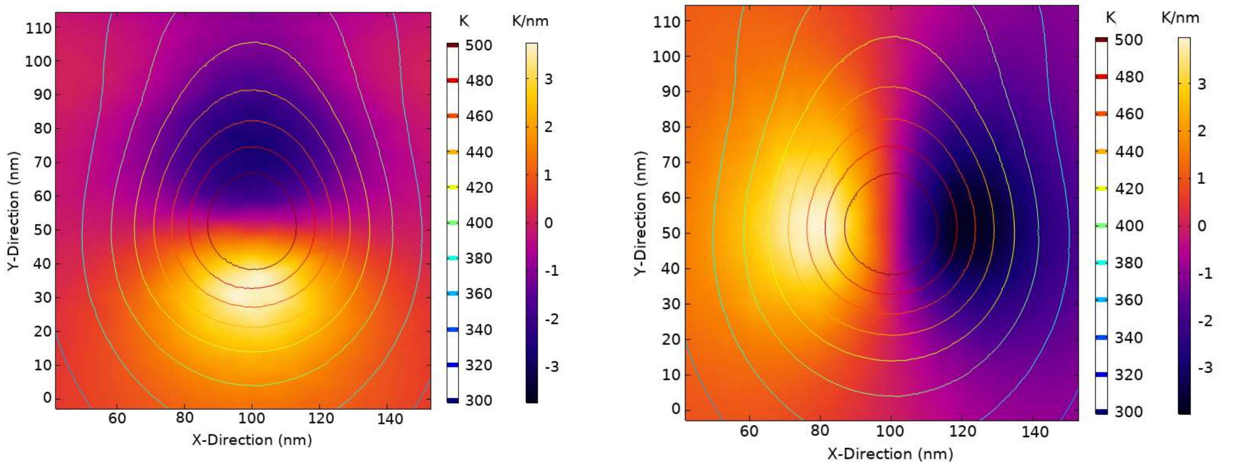


Figure 2 In-plane temperature gradients in the Y- and X-directions for the case of 0.9375 input power are demonstrated with gradients roughly doubled when the power is doubled. Such gradients are necessary in order achieve the changes in temperature required for phonon lasing within the nanoscale region of the QD media. Temperature contours are overlayed which closely resemble the optical field profile.
